# Supplementary material for: Sampling Rare Event Energy Landscapes via Birth-Death Augmented Dynamics
Source: arXiv:2209.00607 ancillary file (2022-12-20)
Supplement: Supplementary file 1 [file SM_BirthDeathAugmentedDynamics.pdf]

# Supporting Material for: Sampling Rare Event Energy Landscapes via Birth-Death Augmented Dynamics

Benjamin Pampel,[1] Simon Holbach,[2,*] Lisa Hartung,[2,†] and Omar Valsson[1,3,‡]

[1] *Max Planck Institute for Polymer Research, Ackermannweg 10, 55128 Mainz, Germany*

[2] *Institut für Mathematik, Johannes Gutenberg-Universität Mainz, Staudingerweg 9, 55099 Mainz, Germany*

[3] *Department of Chemistry, University of North Texas, Denton, TX, USA*

(Dated: December 20, 2022)

**CONTENTS**


S-I. Test of the assumptions of Theorem 2 — 2

S-II. Momentum equilibrium in the general Langevin case — 4

S-III. Effect of varying the birth-death rate factor $\tau_\alpha$ — 6

S-IV. Influence of the number of particles $N$ on the critical bandwidth $\sigma_{\text{crit}}$ — 8

S-V. Additional figures for the comparison between approximations $\Lambda$ — 10

S-V.1. Probability picture — 10

S-V.2. Figures for $\Lambda^{\text{ad}}$ in the overdamped case — 11

S-VI. Behavior for large kernel bandwidths — 13

S-VII. Recalculation of birth-death probabilities for $M = 10,000$ — 15

S-VIII. Additional simulations with the 2D Wolfe-Quapp potential — 17

S-VIII.1. Simulations with 100 particles — 17

S-VIII.2. Simulations with scaled WQ potential — 17

S-IX. Influence of the choice of Langevin time step $\theta$ — 21

References — 23


## S-I. TEST OF THE ASSUMPTIONS OF THEOREM 2

Although there is currently no hard proof that the assumptions of Theorem 2 of the main text hold for the potentials we treat, we can nevertheless evaluate if these are satisfied during the simulations. Here we look more closely at the second assumption of the theorem: There is a $\lambda' > -D\lambda/\tau_\alpha$ such that

$$\text{Cov}_{\rho_t}\left(\log\frac{\rho_t}{\pi}, \log\frac{K*\rho_t}{K*\pi}\right) \geq \lambda' D_{\text{KL}}(\rho_t|\pi) \tag{S1}$$


* s.holbach@uni-mainz.de

† lhartung@uni-mainz.de

‡ omar.valsson@unt.edu

for all $t > 0$, where

$$\mathrm{Cov}_\rho(f, g) = \int fg\rho\,\mathrm{d}x - \int f\rho\,\mathrm{d}x \int g\rho\,\mathrm{d}x. \tag{S2}$$

To evaluate if this assumption holds, we calculate

$$\lambda'_{\min}(t) = \frac{\mathrm{Cov}_{\rho_t}\left(\log\frac{\rho_t}{\pi}, \log\frac{K*\rho_t}{K*\pi}\right)}{D_{\mathrm{KL}}(\rho_t|\pi)} \tag{S3}$$

for the time series of a simulation and see if there is a lower bound. We perform a simulation with the overdamped Langevin solver on the one-dimensional double-well potential also used in Sec. IV of the main text and defined in Eq. (50). We distribute 100 particles randomly in the range $x \in [-2.5, 2.5]$ and run the simulation for 100,000 time steps of length $\theta = 0.001$ with $D = \beta = 1$. The birth-death evaluations are performed according to $\Lambda^{\mathrm{mu}}$ every $M = 100$ steps using a kernel width of $\sigma = 0.4$. To calculate the terms of eq. (S3) we need to first estimate $\rho_t$ from the particle distributions. Similar as in the birth-death algorithm, we use a kernel density estimation with a bandwidth of $\sigma = 0.4$. The integrations for the covariance and Kullback-Leibler divergence are then performed on a grid with 50 points. The resulting time series is shown in Figure S1.

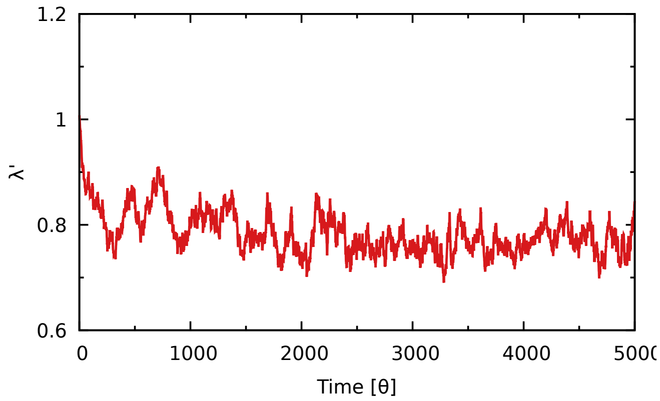


FIG. S1. Evaluation of $\lambda'_{\min}$ via eq. (S3) for the time series of an exemplary simulation. Shown are only the first 5,000 time steps.

Looking at the resulting values of $\lambda'_{\min}$, we observe only minor fluctuations after some short initial transient where the value declines from around 1 to roughly 0.8. This suggests that $\lambda'_{\min}$ has a positive lower bound. In particular, it seems plausible that the assumption of eq. (S1) is satisfied with $\lambda' = 0$, as is also the case when no smoothing kernel is applied at all.

## S-II. MOMENTUM EQUILIBRIUM IN THE GENERAL LANGEVIN CASE

In the general Langevin case, we chose to still have the birth-death rates depend only on the particles' positions and not on their momenta. This approach is valid, if it does not severely disturb the distribution of the momentum. We expect this not to be the case when the momenta equilibrate on timescales shorter than the average time between accepted birth death events.

We verify this by looking at the time evolution of the momenta as well as their distribution. For this, we use data from the simulation with the general Langevin solver and the one-dimensional double-well system with the lowest barrier presented in Sec. IV C of the main text. The momenta of all particles from the first 200,000 time steps are collected into a histogram with 1,000 bins in the range $[-5, 5]$, which is subsequently compared to the expected distribution after normalization.

The theoretical equilibrium distribution of the momentum is given by the Maxwell-Boltzmann distribution in one dimension [1]:

$$\phi(p) = \sqrt{\frac{\beta}{2\pi m}} \exp\left(\frac{-\beta p^2}{2m}\right) \tag{S4}$$

A plot of the probability distributions can be seen in Fig. S2(a). We observe good agreement of our data and the expected equilibrium distribution.

To further verify that our approach does not distort the momentum distribution, we take a look at the relevant timescales. We define the autocorrelation function of the momentum as

$$Z(\tau) = \langle p(\tau) \cdot p(0) \rangle, \tag{S5}$$

with the lag time $\tau$ and the average running over the time series of a single particle within a simulation. We calculate the momentum autocorrelation from the first 200,000 time steps of the simulation data for selected particles. The results are very similar for all chosen particles, we show one exemplary function in Fig. S2(b). We also note that we could not spot significant differences to autocorrelation functions calculated from pure Langevin dynamics simulations of the same system.

The momentum autocorrelation decays to zero within a few hundred Langevin time steps. We compare this time scale of momentum equilibration to the average time between accepted birth-death events. During the simulation, birth-death moves are attempted after

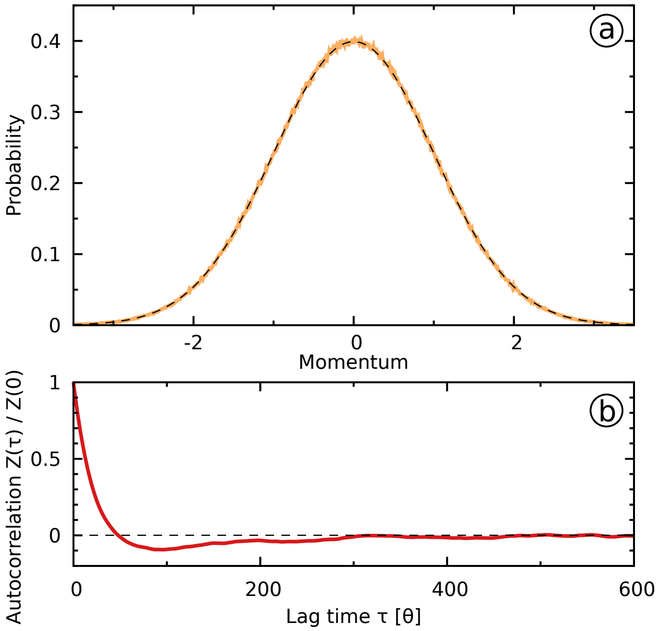


FIG. S2. (a) Momentum distribution from the simulation (solid line) compared to the expected Maxwell-Boltzmann distribution (dashed line). (b) Autocorrelation function of the momentum of one selected particle. The lag time is given in units of the time step.

every 100th Langevin time step, of which 1.67 % are accepted. The average time between birth-death moves is therefore roughly 6,000 Langevin time steps. This is more than one order of magnitude larger than the time required for the momentum to equilibrate. We conclude that the birth-death events have no noticeable effect on the momentum distribution. Therefore the presented approach of Algorithm 1 of the main text is justified even with general Langevin dynamics in the presented case.

## S-III. EFFECT OF VARYING THE BIRTH-DEATH RATE FACTOR $\tau_\alpha$

To avoid cross-effects from varying another parameter, the main text used only simulations with a birth-death rate factor of $\tau_\alpha = 1$. Here we will present additional simulations of the one-dimensional double-well system used in Sec. IV of the main text and defined in Eq. (50). Besides varying the rate factor $\tau_\alpha$, we keep the same simulation protocol as in that section: We use 100 particles with an initial distribution of 10 in the left metastable state at $x_L = -1.4$ and 90 in the right one $x_R = +1.4$. We run a total of 2,000,000 Langevin steps with a time step of $\theta = 0.001$ and $D = \beta = 1$. Every 100 Langevin steps, we calculate the birth-death probabilities via the approximation $\Lambda^{\mathrm{mu}}$ and execute the respective accepted events. We show the resulting distribution of the particles in the two states, as well as the percentage of accepted birth-death events in Fig. S3. The rate of accepted birth-death events $p_{\mathrm{acc}}$ is calculated by counting the number of executed birth-death steps during the simulation and dividing it by the total number of attempted birth-death moves.

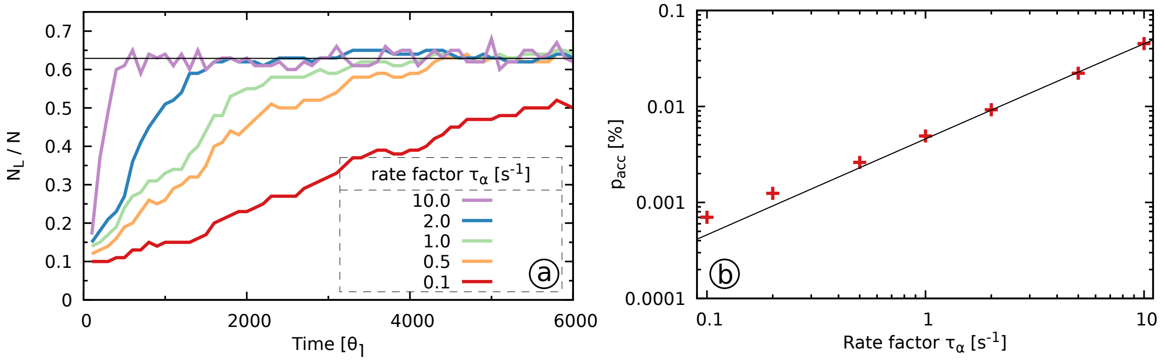


FIG. S3. Effect of different rate factors $\tau_\alpha$ for the birth-death term.
(a) Number of particles in the left state as a function of simulation time for the different rate factors $\tau_\alpha$. Shown are only the first 6,000 time steps. The solid black line is the equilibrium value calculated from the potentials. (b) Percentage of accepted birth-death events from the total number of birth-death events. The log-log representation is only for the purpose of including a wider range of data and has no other meaning. The solid black line shows an approximation of the form $p_{\mathrm{acc}} = 1 - \exp(a * \tau_\alpha)$ to the data.

Looking at the time evolution of the particle distributions in the two states, using a higher rate factor results in reaching the expected equilibrium value faster during the initial steps of the simulation. After equilibration, higher rate factors result in slightly larger fluctuations

around this value, although the effect is not significant in the investigated range. The fraction of accepted birth-death events $p_{\text{acc}}$ can be treated as an approximation of the average birth-death probability

$$1 - \exp\left(-\tau_\alpha |\Lambda_i| M\theta\right). \tag{S6}$$

When we are increasing the rate factor, the birth-death probabilities are also increased in near linear fashion ($1 - \exp(ax) \approx ax$ for $x \ll 1$). Approximating the data with an exponential fit according to Eq. (S6) as shown in Fig. S2(b) shows that the general trend is indeed correct, although some slight deviations for lower $\tau_\alpha$ are visible. In the limit of $\tau_\alpha \to 0$ the birth-death process is turned off completely. Further investigation into the behavior at extreme rate factors will be necessary to fully understand the associated mechanisms.

## S-IV. INFLUENCE OF THE NUMBER OF PARTICLES $N$ ON THE CRITICAL BANDWIDTH $\sigma_{\text{crit}}$

In the main text, we performed all simulations of 1D potentials with 100 particles and all simulations of 2D potentials with 1,000 particles. We found that there seems to be a critical kernel bandwidth $\sigma_{\text{crit}}$ below which the sampling is no longer accurate in the high-energy regions. Its dependence on the potential is hard to investigate systematically, but we can show the influence of the number of particles for a given system in the following simulations. We used the simulation protocol for the overdamped Langevin integrator and the simple 1D potential of Sec. IV A with 10, 30, 300, and 1,000 particles. For each fixed number of particles we iterated over the bandwidth in the range $\sigma \in [0.05, 0.75]$ in steps of 0.05.

We calculate the Kullback-Leibler divergence $D_{\text{KL}}(\pi|\eta)$ from the obtained sampling probabilities to the true equilibrium for all simulations. In Fig. S4(a) we show the results for each set of simulations with fixed particle number as a function of the bandwidth $\sigma$.

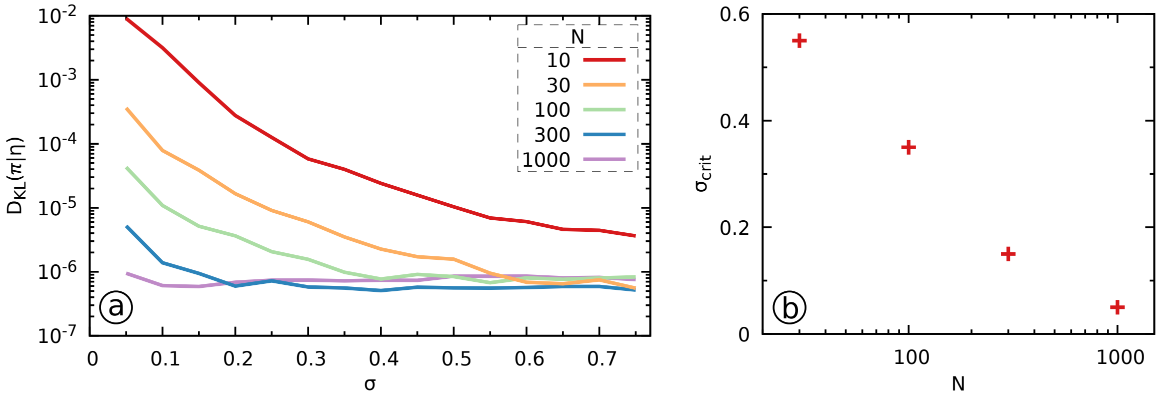


FIG. S4. (a) Kullback-Leibler divergences from the estimated probability distribution to the equilibrium distribution for simulations with different numbers of particles $N$ and bandwidths $\sigma$. (b) Value of the critical bandwidth $\sigma_{\text{crit}}$ defined as the lowest value of $\sigma$ for which $D_{KL}(\pi|\eta) \leq 10^{-6}$ for the simulation series given in part (a). The value for 10 particles is missing as the criterion is never met.

The KL divergence decreases with increasing $\sigma$ for all sets of simulations. At larger $\sigma$ nearly identical values below $10^{-6}$ are obtained for all sets except $N = 10$, which means that sampling very close to the correct distribution is achieved. For the present purpose we define $\sigma_{\text{crit}}$ as the lowest bandwidth at which the threshold $D_{\text{KL}}(\pi|\eta) \leq 10^{-6}$ is achieved.

Figure S4(b) shows the values that were obtained with this criterion. For the simulations with just 10 particles, we could not observe the required sampling accuracy within the range of $\sigma$ under investigation. The value of $\sigma_{\rm crit}$ decreases with increasing number of particles.

This observed effect of a critical bandwidth can be explained by the mechanism of the density estimation used for the birth-death probabilities. A very small bandwidth and a small number of particles lead to a rather spiky density estimate with sparse isolated peaks at the particle positions, while increasing the bandwidth and the number of particles yields a smoother density estimate.

Taking an exponential fit to the obtained critical bandwidth values of Fig. S4(b) yields approximately $\sigma_{\rm crit} \propto N^{-1/2}$. An exponential behavior is in line with the general literature on density estimation from stochastic data, where theoretical values for the relationship between the number of data points and the optimal width of the Gaussian kernel used in the density estimation have been deduced [3], assuming a normal distribution of the data.

We conclude that the parameter $\sigma$ has to be chosen large enough to get a smooth estimate of the density, but further investigation is needed before we can give an a-priori rule-of-thumb.

## S-V. ADDITIONAL FIGURES FOR THE COMPARISON BETWEEN APPROXIMATIONS $\Lambda$

### S-V.1. Probability picture

While we have shown estimates of the energy landscape from our simulations in the main text, an alternative picture is to look at estimates of the corresponding probability density. As this is the representation often chosen in the stochastics community from which the original algorithm of Ref. 2 is coming, we also provide this representation for the results of Section IV A of the main text. Using the same simulation data, we present analogous figures to Fig. 1(a,b) of the main text in Fig S5.

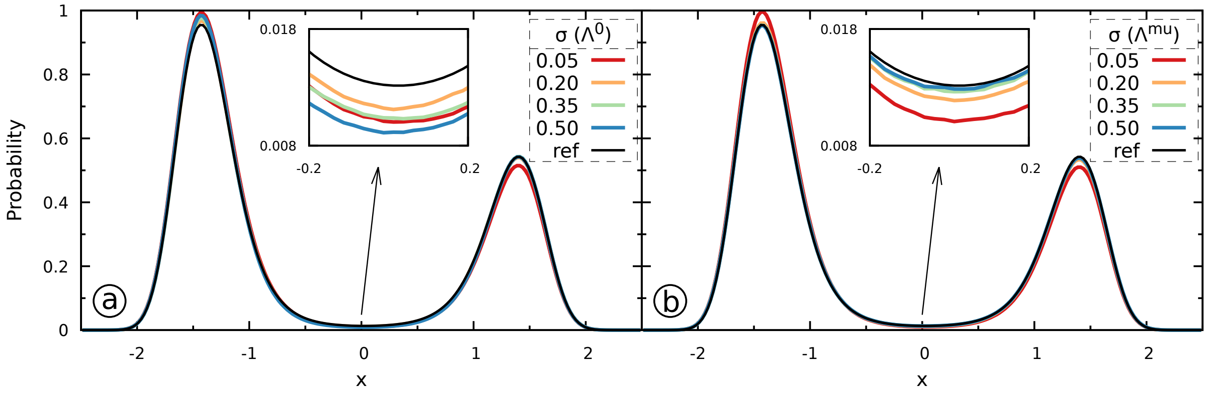


FIG. S5. Estimates of the probability density from simulations using the approximation (a) $\Lambda^0$ and (b) $\Lambda^{\mathrm{mu}}$ and different kernel widths $\sigma$ together with the reference obtained from the potential. The simulation data is the same as in Sec. IV A and Fig. 1 of the main text.

In the energy landscape picture of Fig 1(a,b) of the main text, the barrier around $x = 0$ was estimated to be higher in energy for all simulations with $\Lambda^0$, while this only occurred for small kernel widths with $\Lambda^{\mathrm{mu}}$. In the probability representation of Fig S5 this transfers to an undersampling of the same region. Because this region has very low probabilities, the deviation from the reference in absolute numbers is only very minor and in fact is nearly indistinguishable in the figures. Only when zooming into the region, as it is done in the insets of the figures, the deviation becomes apparent.

This can explain why the issue with the original approximation $\Lambda^0$ was not noticed in Ref. 2. There, the Kullback-Leibler divergence was used as a measure of similarity between probability distributions to estimate the performance of the algorithm. As regions with

small probabilities contribute only to a small extend to the Kullback-Leibler divergence, deviations from the equilibrium sampling in low probability regions are easy to miss in the probability picture.

### S-V.2. Figures for $\Lambda^{\text{ad}}$ in the overdamped case

Although Sec. II B of the main text proposed two new approximations for the birth-death probabilities, only simulations with $\Lambda^{\text{mu}}$ were presented. For comparison, we also performed simulations with $\Lambda^{\text{ad}}$, as defined in Eq. (12) of the main text. The protocol is the same as in Sec. IV A of the main text, i.e. we use overdamped Langevin dynamics to simulate the movement of 100 particles in a simple one-dimensional double-well potential and attempt birth-death moves every 100 time steps. Simulations were done for different values of the bandwidth $\sigma$.

Figure S6(a) shows exemplary energy landscapes obtained from the simulations, while (b) depicts the height of the barrier as a function of the bandwidth for all three approximations. Similar to the results when using the approximation $\Lambda^{\text{mu}}$, we observe good sampling with $\Lambda^{\text{add}}$ if the bandwidth $\sigma$ is chosen large enough. Additionally, we calculated the Kullback-Leibler divergence $D_{\text{KL}}(\pi|\eta)$ to the true equilibrium distribution for all approximations and show the results in Fig. S6(c). The slightly lower values for $\Lambda^{\text{ad}}$ compared to $\Lambda^{\text{mu}}$ are a coincidence that comes from using only a single simulation per data point. The same simulations were repeated with different initial seeds of the random number generator. The results from different runs show fluctuations on the same order as the differences visible here and no clear trend which of the two approximations is better. In the main text we focused on the approximation $\Lambda^{\text{mu}}$ because it provides better properties for mathematical analysis while showing the same behavior in numerical simulations as $\Lambda^{\text{ad}}$.

Concludingly, we obtain sampling very close to the equilibrium distribution for both newly proposed approximations when employing sufficiently large bandwidths.

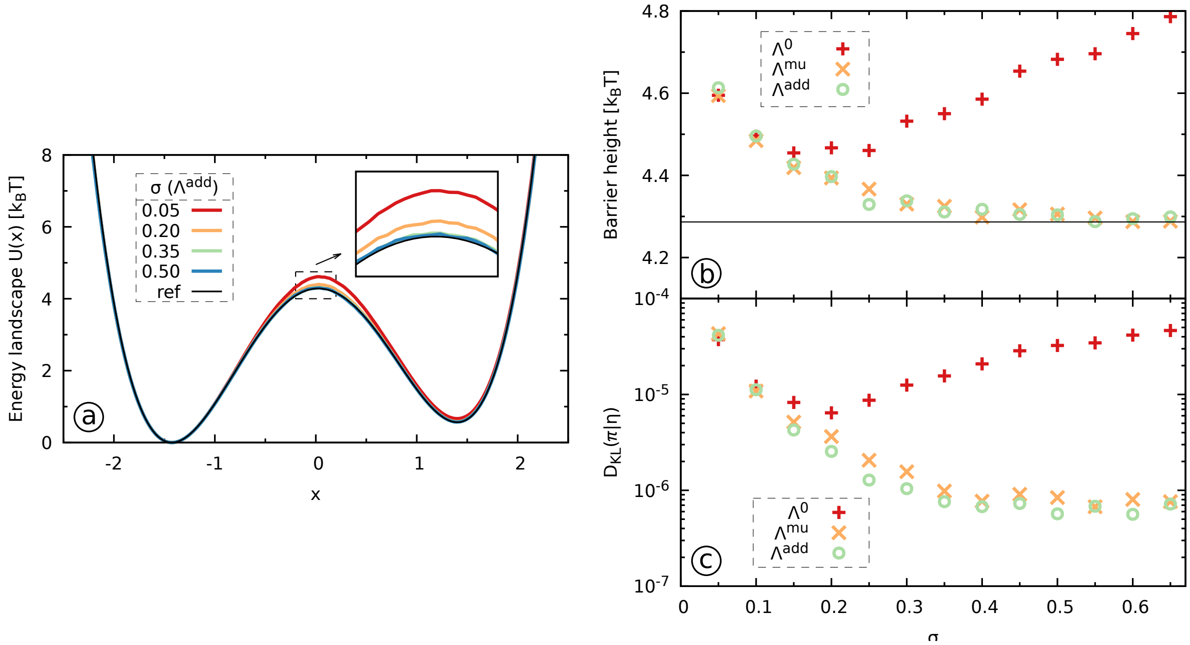


FIG. S6. (a) Estimates of the energy landscape from sampling by using $\Lambda^{\mathrm{add}}$ for the birth-death probabilities. Shown are results for different values of the bandwidth $\sigma$ (colored) as well as the reference (black). The small inset shows a magnification of the barrier region. (b) The height of the barrier from the estimates of the energy landscape as a function of the bandwidth $\sigma$, calculated from the left minimum. The reference value is given as black horizontal line. (c) Kullback-Leibler divergences from the estimated probability distribution to the equilibrium distribution for simulations with different bandwidths $\sigma$ and approximations $\Lambda$.

## S-VI. BEHAVIOR FOR LARGE KERNEL BANDWIDTHS

We noted in Lemma 1 of the main text that the birth-death rates $\Lambda^{\mathrm{mu}}$ go to zero when the bandwidth goes to infinity. This can also be explained intuitively: In the limit of infinite width, the Gaussians locally resemble a uniform distribution, so that the values of the first and second terms in Eq. (47) of the main text are independent of the particle position. Since the third term is the average of these two terms over all particles, the birth-death rates become zero. For our algorithm, this means that we can gradually "turn off" the birth-death part of the dynamics by increasing the bandwidths. In the limit of infinitely wide kernels we perform only pure Langevin sampling.

In order to demonstrate this effect, we perform simulations with the overdamped Langevin solver on the one-dimensional double-well potential also used in Sec. IV of the main text and defined in Eq. (50). The simulation protocol is kept the same: We use 100 particles with an initial distribution of 10 in the left metastable state at $x_L = -1.4$ and 90 in the right one $x_R = +1.4$. We run a total of 2,000,000 Langevin steps with a time step of $\theta = 0.001$ and $D = \beta = 1$. Every 100 Langevin steps, we calculate the birth-death probabilities via the approximation $\Lambda^{\mathrm{mu}}$ and execute the respective accepted events. The width of the Gaussian kernels is varied in the range $\sigma \in [0.5, 5]$ in steps of 0.5. Additionally, we perform one simulation without the birth-death algorithm. We show the resulting distribution of the particles in the two states, as well as the percentage of accepted birth-death events in Fig. S7. The rate of accepted birth-death events $p_{\mathrm{acc}}$ is calculated by counting the number of executed birth-death steps during the simulation and dividing it by the total number of attempted birth-death moves.

Looking at the time evolution of the particle distribution, we find that with increasing bandwidth $\sigma$, the convergence towards the equilibrium distribution takes more and more time. We can see that for the largest values of $\sigma$ the evolution gradually approaches the behavior of the simulation without birth-death, as predicted by the theory. We note that we used the same set of random numbers for the noise term of the Langevin solver in all simulations to reduce differences from the Langevin dynamics, which is visible in the similarity of the time evolution. Looking at the percentage of accepted birth-death events in Fig. S7(b), we observe a reduction of about one order of magnitude between the smallest and largest chosen value of $\sigma$. This exponential decrease confirms the assertion that large

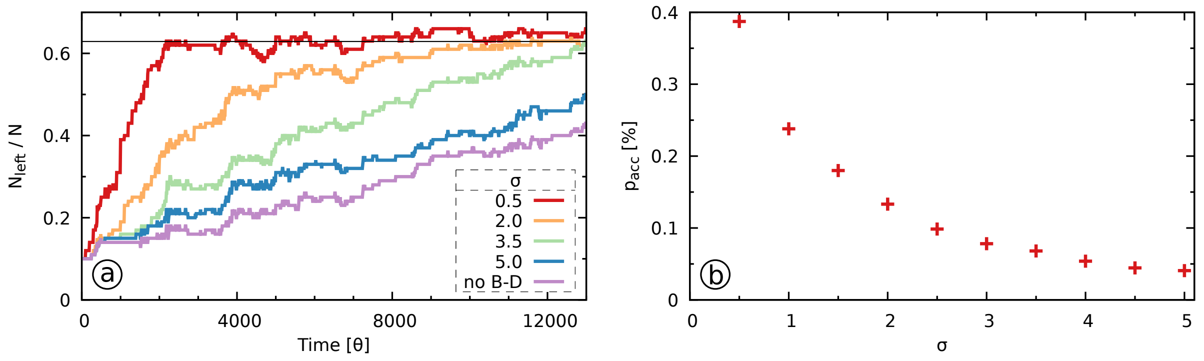


FIG. S7. Effect of choosing large bandwidths on the performance of the birth-death algorithm. (a) Number of particles in the left state as a function of simulation time for the different bandwidths $\sigma$ as well as one simulation without birth-death events. Shown are only the first 13,000 time steps. The solid black line is the equilibrium value calculated from the potentials. (b) Percentage of accepted birth-death events from the total number of birth-death events.

bandwidths can be used to gradually turn off the birth-death algorithm.

## S-VII. RECALCULATION OF BIRTH-DEATH PROBABILITIES FOR $M = 10,000$

In Sec. IV B of the main text, we noted "overshooting" of the particle distribution when performing the birth-death calculations only sparsely, i.e. with more than 1,000 Langevin time steps between attempting birth-death events. We found the combination of high average birth-death probabilities together with the "bulk" calculation of them responsible for this. Here, we will verify this assumption by taking a closer look at the case $M = 10,000$. For this, we found average birth-death probabilities of $p_{\mathrm{acc}} \approx 70\,\%$. The individual probabilities correspond to making a single birth or death move for one particle given the overall distribution of particles. Because we calculate the birth-death probabilities for all particles at the beginning of the birth-death step, the change of the particle distribution as well as the birth-death probabilities after each accepted birth-death event is not taken into account. As long as only few birth-death events occur, the particle distribution does not change significantly during the birth-death step of the algorithm. Looking at the results of Sec. IV B, we can verify that the sampling does not change significantly for $p_{\mathrm{acc}} > 5\,\%$.

To verify that the combination of high average birth-death probabilities together with the bulk calculation and execution of the events is indeed responsible for this, we run an additional simulation with $M = 10,000$ using the same protocol and initial conditions as in Sec. IV B of the main text, but with a slightly modified algorithm: Instead of executing all accepted birth-death events simultaneously, the probabilities are recalculated during the birth-death step whenever an accepted event has been carried out. Hence, the changed particle distribution is taken into account during the course of the birth-death step. The resulting time evolution of the particle distribution can be seen in Figure S8, together with the previous data without recalculation of the probabilities.

Looking at the first birth-death step at $t = 10,000 \cdot \theta$, the fraction of particles in the left state was roughly 0.35 immediately before it. This is far from the equilibrium distribution of 0.63 which results in high probabilities of getting killed for the particles in the right state, and high probabilities of getting duplicated for particles in the left state. When applying the birth-death moves simultaneously for all particles without recalculation of the probabilities in between, this results in "overshooting" such that too many particles transfer to the left state. On subsequent birth-death steps, the same effect is observed, which results in large fluctuations around the mean value.

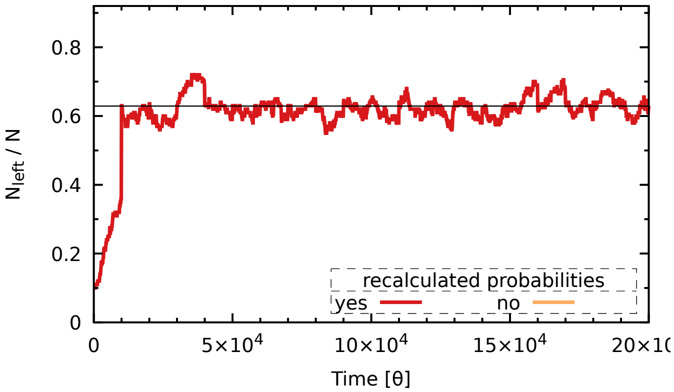


FIG. S8. Effect of recalculating the birth-death probabilities after each accepted birth-death event. Shown is the fraction of particles in the left state as a function of simulation time. The data is for $M = 10,000$ when recalculating the birth-death probabilities after each accepted event (red) or in bulk (orange), the black horizontal line is the expected equilibrium value. Depicted are only the first 200,000 time steps. The orange line is the same data as for the $M = 10,000$ line in Fig. 2(d) of the main text.

For the simulation where the events are applied one at a time and the probabilities are recalculated in case of success, this "overshooting" effect does not occur and the birth-death step results in particle distributions close to the equilibrium. To assess the change numerically, we calculate the same values as in Sec. IV B, namely the rate of accepted birth-death events $p_{\mathrm{acc}}$ and the standard deviation of the fraction of particles in the left states. The average birth-death probability decreases significantly from $p_{\mathrm{acc}} = 0.68$ to $p_{\mathrm{acc}} = 0.21$, and the standard deviation as a measure of the fluctuation of $N_{\mathrm{left}}/N$ shrinks from 16.4 to 3.3. The per-particle approach with recalculation of the probabilities after each accepted event thus solves the problem of overshooting but requires a lot more computational effort. As long as the birth-death probabilities are small, the approach of the main text is justified and should be used for better efficiency.

## S-VIII. ADDITIONAL SIMULATIONS WITH THE 2D WOLFE-QUAPP POTENTIAL

### S-VIII.1. Simulations with 100 particles

In the main text, we showed results for simulations with 1,000 particles on the two-dimensional Wolfe-Quapp potential defined in Eq. (53) of the main text. Here, we present additional simulations with a similar protocol but only 100 particles. To get the same amount of data points, we increase the number of time steps by a factor of 10, resulting in 2,000,000 steps. While this allows for a good comparison of the estimates, the overall longer simulation time results also in increased observability of long-time behavior, such as rare transitions between the states. An analogous figure to Fig. 4 of the main text can be seen in Fig. S9. Looking at the projection of the energy landscapes on the y-axis in part (b), we see that larger values of the bandwidth $\sigma$ are required for a good estimate than with 1,000 particles. In fact, we performed simulations with values up to $\sigma = 1.0$ to get adequate results. While the smallest shown value $\sigma = 0.1$ is significantly off, we observe that the simulation without birth-death yields a better estimate than with 1,000 particles. This is due to the longer simulation times per particle and the saddle point height of only around $5\,k_{\mathrm{B}}T$, which results in barrier crossings on long time scales. In Fig. S9(c), we confirm the approximately correct sampling for large bandwidths $\sigma$. In comparison to the simulations with 1,000 particles, larger bandwidths are needed, which agrees with the findings in Sec. S-IV. Looking at Fig. S9(d), we observe similar time scales until the particles have equilibrated in the two states when using birth-death moves. The fluctuations around the equilibrium are more prominent due to the smaller number of particles.

### S-VIII.2. Simulations with scaled WQ potential

When running simulations with the original Wolfe-Quapp potential given in Eq. (53) of the main text, we could still observe transitions between the two main states from the Langevin dynamics, which was especially apparent for the longer simulation times with 100 particles that were presented in the previous section S-VIII.1. To test the algorithm also with a "true" rare-event system, we additionally perform simulations on a scaled version,

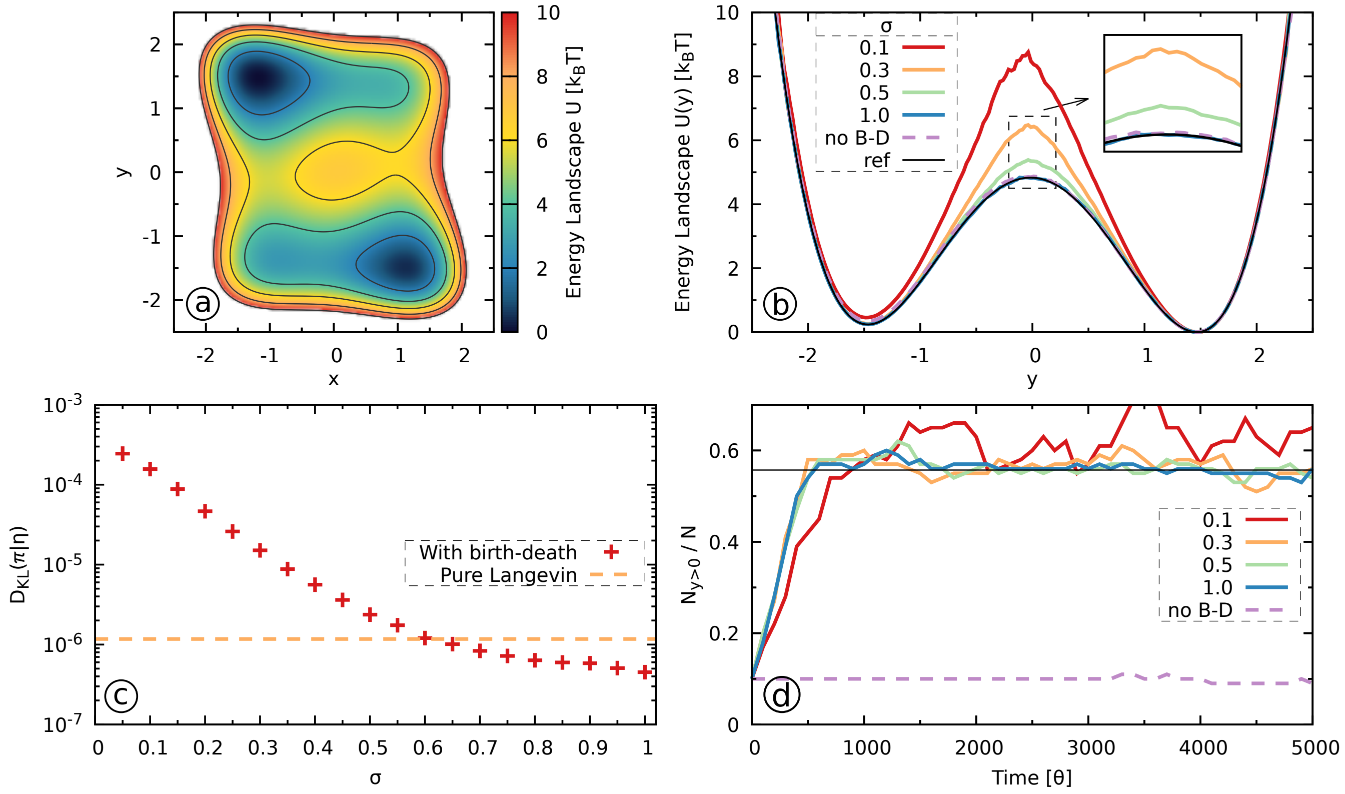


FIG. S9. (a) The reference energy landscape of the Wolfe-Quapp potential. (b) Estimates of the energy landscape projected on the y-direction. Colored solid lines are from simulations with 100 particles with birth-death events using different bandwidths $\sigma$. We note that the blue line stands here for $\sigma = 1.0$, different than in the figure with 1,000 particles in the main text. The dashed line is from a pure Langevin dynamics simulation with 100 particles. The black line is the expected energy landscape calculated from the potential. (c) Kullback-Leibler divergences from the estimated probability distribution to the equilibrium distribution for simulations with different bandwidths $\sigma$. For comparison, the dashed horizontal line is from a simulation without the birth-death algorithm. (d) Number of particles in the state with $y > 0$ as a function of simulation time. The black horizontal line is the expected equilibrium value. The different lines represent the same simulations as in (b).

given by the mathematical expression

$$U(x, y) = 3x^4 + 3y^4 - 6x^2 - 12y^2 + 3xy + 0.9x + 0.3y. \tag{S7}$$

This is the original Wolfe-Quapp potential scaled by a factor of 3.

For this potential, we conduct simulations with an otherwise identical protocol as in

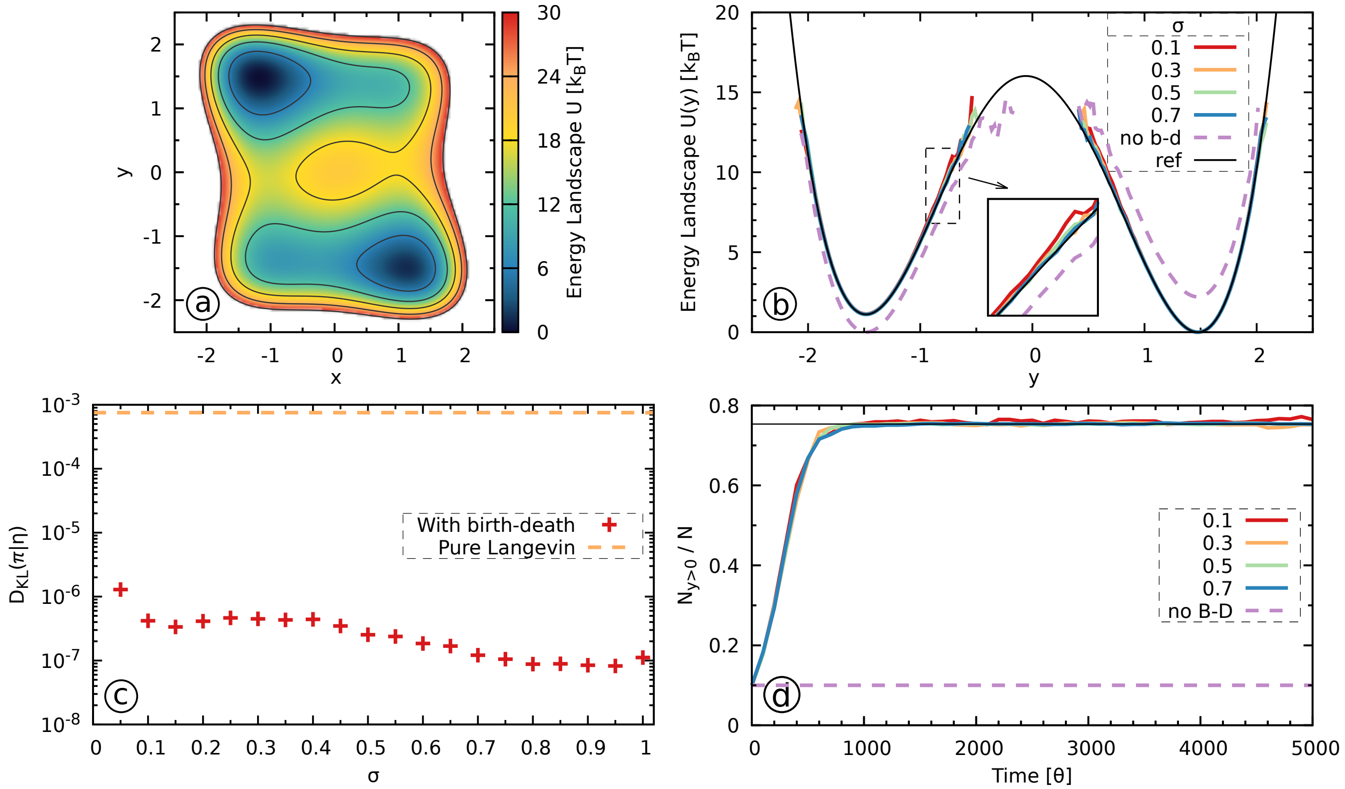


FIG. S10. (a) The reference energy landscape of the scaled Wolfe-Quapp potential eq. S7. (b) Estimates of the energy landscape projected on the y-direction. Colored solid lines are from simulations with 1,000 particles with birth-death events using different bandwidths $\sigma$. We note that even in the magnified inset the lines are hardly distinguishable because they basically are on top of each other. The dashed line is from a pure Langevin dynamics simulation with 1,000 particles. The black line is the expected energy landscape calculated from the potential. (c) Kullback-Leibler divergences from the estimated probability distribution to the equilibrium distribution for simulations with different bandwidths $\sigma$. For comparison, the dashed horizontal line is from a simulation without the birth-death algorithm. (d) Number of particles in the state with $y > 0$ as a function of simulation time. The black horizontal line is the expected equilibrium value. The different lines represent the same simulations as in (b).

Sec. IV D of the main text. In particular we resume to $N = 1,000$ particles. Results are shown in Fig. S7. Looking at the exemplary projections of the energy landscape in part (b) of the figure we observe that the simulations with birth-death events are capable of sampling this two-dimensional system correctly. On the contrary, the estimate from pure Langevin

sampling does not get the energy difference between the states correctly, but only the local shapes of the two basins. This is also visible from the Kullback-Leibler divergence to the reference distribution given in Fig. S10(c), which is three orders of magnitude larger than for the simulations with birth-death events. For these we observe the same general trend as for the simulations with the original Wolfe-Quapp potential: with increasing bandwidth the Kullback-Leibler divergence goes down until it reaches a plateau. This plateau is not as clearly visible as before, which we blame on the strong emphasis of the KL divergence on the most likely states. Only the region directly around the two states lowest in energy contributes significantly to the calculation of the KL divergence for this system, such that small differences in these regions can result in notable differences. Generally, we conclude that pure Langevin dynamics is not capable of sampling this system adequately, which we can cure by introducing birth-death events.

## S-IX. INFLUENCE OF THE CHOICE OF LANGEVIN TIME STEP $\theta$

All of our simulations so far use a time step of $\theta = 0.001$ for the overdamped Langevin case and a time step of $\theta = 0.005$ for the general Langevin case. To assess if our choice of the time steps is responsible for some of the effects we observed, we also performed simulations with different time steps for both the overdamped and the general Langevin case.

As a test system we choose 100 particles in the simple one-dimensional potential that was introduced in Eq. (50) of the main text. To reduce effects from the suppressed transitions between the two states, we choose to start out with a distribution of the particles close to the equilibrium, that is 63 particles at $x_L = -1.4$ and 37 at $x_R = 1.4$.

We run for 2,000 time units in total with four different Langevin time steps for both the overdamped and the general Langevin case: $\theta = 0.1, 0.01, 0.001, 0.0001$. In the overdamped case, we set $D = \beta = 1$, while in the general case we set $k_{\mathrm{B}}T = 1$, $m = 1$, and $\gamma = 10$. For both cases, we run simulations with and without the additional birth-death steps. The simulations with birth-death steps use a bandwidth of $\sigma = 0.5$, which has worked well in our previous simulations. We choose to attempt birth-death events after every 0.1 time units for all simulations.

In the overdamped case, the simulations with $\theta = 0.1$ turned out to be instable. Due to the large timestep, the particles were able to move distances much larger than the wells of the two states within one step. This lead to particles reaching states with very high energies at the edges of the system. Due to the shape of the potential, the force towards the center increases roughly cubic with the distance to the center of the system. In the next time step, the large force associated with the previous state far up the outer wall moves the particle a large distance into the opposite direction. Eventually, the particle can continue to "bounce" off the walls at the two edges to reach increasingly high energy states. This is not representing the desired sampling of the system. We therefore conclude that $\theta = 0.1$ is too large for this system when using the overdamped Langevin integrator.

For all other simulations, we analyze the results further. After removing the first 10 time units of the trajectories, all intermediate particle positions are used to evaluate the correct sampling via histogramming. The energy landscapes corresponding to the histograms can be seen in Fig. S11.

Looking at the overdamped dynamics in Fig. S11(a,b), we observe small deviations from

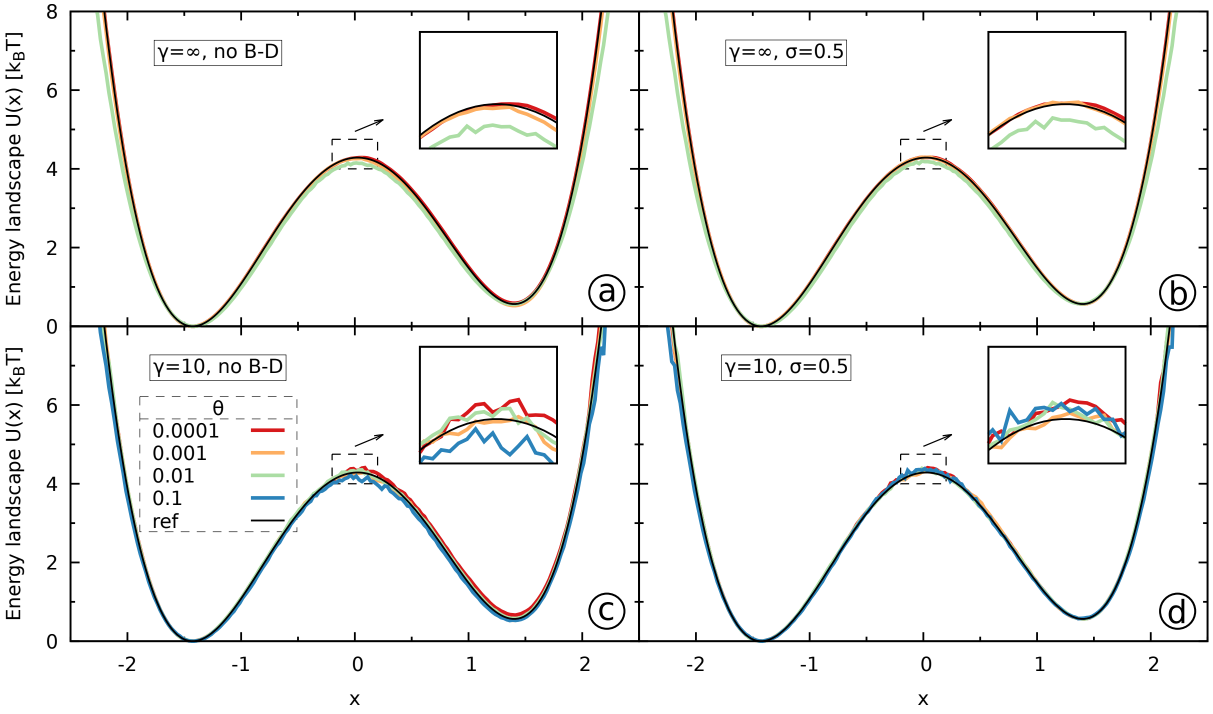


FIG. S11. Energy landscapes estimated from the particle positions simulated with the overdamped Langevin scheme (top, $\gamma = \infty$) and general Langevin scheme (bottom, $\gamma = 10$) for both pure Langevin simulations (left) and simulations with added birth-death steps (right). All plots show results for different values of the Langevin time step $\theta$. The figures for the overdamped Langevin simulations do not display the results for $\theta = 0.1$ as these simulations were instable and did not return meaningful estimates.

the correct sampling at the barrier for $\theta = 0.01$. For smaller time steps, such as the $\theta = 0.001$ used in all other simulations, we observe good agreement with the reference from the potential. We cannot spot differences between pure Langevin sampling in Fig. S11(a) and the sampling with added birth-death steps in (b).

The resulting energy landscapes for simulations with the general Langevin integrator are displayed in Fig. S11(c,d). In the case of pure Langevin sampling in (c), the height of the barrier is slightly underestimated for $\theta = 0.1$. For smaller time steps no significant differences can be observed at the barrier, although the smallest value ($\theta = 0.0001$) is slightly overestimating the height of the right minimum. When adding birth-death steps in (d), no differences to the reference energy landscape, except for some random fluctuations due to the finite sampling, are observed.

Concludingly, the choices of time step for both the overdamped and the general Langevin simulations presented in the main text fall into the range of approximately correct sampling for the system at hand.

---


[1] David Chandler. *Introduction to Modern Statistical Mechanics.* Oxford University Press, New York, 1987.

[2] Yulong Lu, Jianfeng Lu, and James Nolen. Accelerating Langevin Sampling with Birth-death. *arXiv:1905.09863 [cs, math, stat]*, May 2019.

[3] B. W. Silverman. *Density Estimation for Statistics and Data Analysis.* Number 26 in Monographs on Statistics and Applied Probability. Chapman & Hall/CRC, Boca Raton, 1998.
